# Supplementary material for: Measuring well quasi-ordered finitary powersets
Source: arXiv:2312.14587 source file (2026-12-03)
Supplement: Supplementary file 1 [file appendix-with-omega.tex]

\section{Appendix to
  \cref{sec:up-lower-bounds}
  ``Upper and lower bounds''
 }

\subsection{Structural lemmas}
%-----------------------------
\label{app:proof:mot-sum}

\motsum*
\begin{proof}
	Let $X$ be a \wqo.
	Let $f: \alpha+\beta \rightarrow X$ be a
	maximal linearization of $\le$.
	We let
	$X_\alpha = f([0,\alpha[)$ and $X_\beta = f([\alpha,\alpha+\beta[)$.
	We further assume that $f$ makes $\o(X_\alpha)$ minimal; since the
	collection of all maximal linearization is a set, the collection of
	all possible $\o(X_\alpha)$ is a set of ordinals, which admits a
	minimal element.

	Now, since $f$ is a linearization, for all $a\in X_\alpha, b\in X_\beta$, $a\not\geq b$. It follows that
	\[
		X_\alpha + X_\beta \geqaug X \geqaug X_\alpha \sqcup
		X_\beta
	\]
	which implies:
	$\o(X_\alpha) + \o(X_\beta) \le \alpha + \beta \le \o(X_\alpha) \oplus \o(X_\beta)$.
	Besides, $f$ gives a linearization from $\alpha$ to $X_\alpha$, and one from $\beta$ to $X_\beta$, hence
	$\o(X_\alpha) \ge \alpha$ and $\o(X_\beta) \ge \beta$.
	But then
	$\alpha + \beta \ge \o(X_\alpha) + \o(X_\beta) \ge \alpha + \o(X_\beta)$
	and therefore $\o(X_\beta) = \beta$.
	Besides, since $\o(X_\alpha) \ge \alpha$, it can be written
	$\o(X_\alpha) = \alpha + \gamma$ for some $\gamma$ that must satisfy
	$\gamma + \beta = \beta$.

	Now since $X_\beta$ is upward-closed, concatenating any linearization
	of $X_\alpha$ with one of $X_\beta$ gives one of $X$
	(since $\forall (y,z) \in X_\alpha \times X_\beta, z \not\le y$).
	We consider the linearization $f'$ from
	$\alpha + \gamma + \beta = \alpha + \beta$ to $X$ obtained from
	concatenating two maximal linearization of $X_\alpha$ and $X_\beta$.
	If $\gamma \neq 0$, $Y_\alpha \defined f'([0,\alpha[)$ is a strict subset of
	$X_\alpha$, such that $\o(Y_\alpha) \ge \alpha$, that is
	$\o(Y_\alpha) = \alpha + \delta$ but
	$\alpha + \delta + \gamma = \alpha + \gamma$.
	It follows that $\delta < \gamma$ and
	that $\o(X_\alpha)$ was not minimal, which is absurd.
	Therefore, $\o(X_\alpha) = \alpha$ and the theorem is proved.
\end{proof}

%\begin{proof}[Proof of \cref{pr:prop:width-sub}]
%	By induction on $\w(X)$, $\alpha$ being fixed.
%	\begin{itemize}
%		\item[Base case:] $\w(X) = \alpha$. Then $Y \defined X$
%		      is a solution.
%		\item[Successor:]
%		      $\w(X) = \beta + 1$ and $\w(X) > \alpha$.
%		      Using the \kref{descent-equations}{descent equation},
%		      there exists a $x \in X$ such that
%		      $\w(\ResW{X}{x}) = \beta$.
%		      By induction hypothesis since $\beta \geq \alpha$,
%		      there exists a substructure $Y$ of $\ResW{X}{x}$
%		      such that $\w(Y) = \alpha$. Notice that $\ResW{X}{x}$
%		      is itself a substructure of $X$, hence $Y$ is a substructure
%		      of $X$ of width $\alpha$.
%		\item[Limit:]
%		      $\w(X)$ is a limit ordinal and $\w(X) > \alpha$.
%		      Using the \kref{descent-equations}{descent equation},
%		      $\w(X) = \sup_{x \in X} (\w(\ResW{X}{x}) + 1) > \alpha$.
%		      As a consequence, there exists
%		      $x \in X$ such that $\w(\ResW{X}{x}) \geq \alpha$
%		      and $\w(\ResW{X}{x}) < \w(X)$. We conclude
%		      by induction as in the successor case. \qedhere
%	\end{itemize}
%\end{proof}

\hsum*
\begin{proof}\label{proof:h-sum}
	Below for a \wqo $(X,\le)$ and $x \in X$
	we denote by $\rk_X(x)$ the rank of $x$ inductively defined by
	$\rk_X(x) = \sup_{y < x} (\rk_X(y) + 1)$.
	Alternatively, $\rk_X(x) = \h(X_{<x})$.

	Define $X_\top = \rk_X^{-1}([\alpha,\alpha+n[)$ and
	$X_\bot = X \setminus X_\top$. Using the \kref{descent-equations}{descent equation}, observe that $\h(X_\bot)=\sup_{x\in X_\bot} \h(X_{<x})= \alpha$ and $\h(X_{\top})=n$.
	Let $S = S_\top \cup S_\bot$ and $T = T_\top \cup T_\bot$
	be two elements of $\Pf(X)$, with $S_\top,T_\top\subseteq X_\top$ and $S_\bot,T_\bot\subseteq X_\bot$.
	If $S \hoarele T$, then
	either $S_\top \hoareeq T_\top$, and $S_\bot \hoarele T_\bot$,
	or $S_\top \hoarele T_\top$.
	This proves that $\Pf(X)$ is a substructure of
	$\Pf(X_\bot) \cdot \Pf(X_\top)$.
\end{proof}

\structuralwidth*
\begin{proof}
	\label{proof:successor-width}
	If $n=0$ it's obvious ($\Gamma_0 = \emptyset$).

	$\w(X) = \sup_{x \in X} (\w(X_{\perp x}) + 1)$, therefore there exists
	$x_1$ such that $\w(X_{\perp x}) = \alpha + (n-1)$.
	By induction, we get an antichain $x_1, \dots, x_n$ such that
	$\w(X_{\perp x_1, \dots, x_n}) = \alpha$.
	Take $Y = X_{\perp x_1, \dots, x_n}$.
	and map $\Gamma_n$ to
	$x_1, \dots, x_n$.
\end{proof}

\subsection{Lower bounds on the width of a product}

\begin{definition}
	A wqo $X$ is \emph{transferable} if
	for every $x_1, \dots, x_n \in X$,
	$\w(X \setminus \dwc_\leq \{ x_1, \dots, x_n \}) = \w(X)$
\end{definition}

\begin{proposition}
	\label{indecomp-transf2}
	If $\w(X) \ge \omega$ is additively indecomposable, then $X$ has a substructure of width
	$\w(X)$ which is transferable.
\end{proposition}

\begin{proof}
	By induction on $\h(X)$.
	Since $\w(X) \ge \om$, $X$ is infinite and thus
	$\h(X) \ge \omega$.

	If $\h(X) = \omega$ then for every $x_1, \dots, x_n \in X$,
	$X_1 = \dwc \{ x_1, \dots, x_n \}$ is finite and therefore of finite
	width. It follows that $X_2 \defined X \setminus X_1$ is of width
	$\w(X)$ since the latter is additively indecomposable and
	$\w(X) \le \w(X_1) \oplus \w(X_2)$. That is, $X$ is transferable.

	If $\h(X) > \omega$, either $X$ is transferable, in which case the
	proposition is proved, or there exists $x_1, \dots, x_n \in X$ such
	that $\w(X_2) < \w(X)$ where $X_2 \defined X \setminus X_1$ and
	$X_1 \defined \dwc \{ x_1, \dots, x_n \}$.
	Since $\w(X)$ is additively indecomposable and $\w(X) \le \w(X_1) \oplus \w(X_2)$,
	it follows that $\w(X_1) = \w(X)$. But $\h(X_1) < \h(X)$ by the \kref{descent-equations}{descent equation}, and therefore by induction $X_1$ has a transferable substructure of
	width $\w(X_1) = \w(X)$.
\end{proof}

\begin{corollary}
	\label{cor-indecomp}
	If $\alpha$ is indecomposable, infinite and $\alpha \le \w(X)$ then
	$X$ has a transferable substructure of width $\alpha$.
\end{corollary}

In \cite{dzamonja2020}, there is the following property:
\begin{lemma}
	If $\delta$ is an ordinal and $B$ a transferable WQO, then
	$\w(\delta \times B) \ge \w(B) \cdot \delta$.
\end{lemma}
This lemma can be generalized to any wqo $A$ such that $\o(A)=\delta$.
\begin{lemma}
	\label{lem:fam:bi-transferable-product}
	\label{lbiftransferable}
	Suppose that $A$ is a transferable wqo and $B$ any wqo. Then $\w(A\times B)\geq \w(A)\cdot\o(B)$.
\end{lemma}
\begin{proof}
	This is a generalisation of  \cite[Theorem 4.16]{dzamonja2020}
	which states that for any transferable wqo $A$, and any ordinal
	$\gamma$, $\w(A\times\gamma)\geq \w(A)\cdot \gamma$.
	Let $B$ be a wqo, and $\gamma = \o(A)$. Since $B\leqaug \o(B)$, $\w(A\times B)\geq \w(A\times\o(B))\geq \w(A)\cdot \o(B)$.
\end{proof}

\lbiftransferable*
\begin{proof}[Proof of \cref{lem-isa}]
	\label{proof:lem-isa}
	Since $\w(B)$ is indecomposable, it has a substructure $C$ of width
	$\w(B)$ which is transferable (proposition above).

	Hence $A\times B \geqstruct A \times C$ and $\w(A\times B)\geq \w(A\times C) \geq \w(B)\cdot \o(A)$ according to \cref{lbiftransferable}.
\end{proof}

\section{Appendix to
  \cref{sec:tightness}
  ``Tightness of the bounds''
 }

\sumequalssupordinals*
\begin{proof}
	\label{proof:sum-equals-sup-ordinals}
	We now prove the result by induction on $\alpha > 0$.
	\begin{itemize}
		\item[For $\alpha = 1$] we have $1 = \om^{\alpha-1}$.

		\item[For $\alpha = \gamma+1$, $\gamma$ limit ordinal] we have:
		      \begin{equation*}
			      \sum_{\beta < \alpha} \om^{\beta}
			      = \sum_{\beta < \gamma} \om^{\beta} + \om^\gamma =
			      \omega^\gamma +
			      \omega^\gamma
			      = \om^{\alpha - 1} \cdot 2 \, .
		      \end{equation*}
		\item[For $\alpha = \gamma+2$] we have:
		      \begin{align*}
			      \sum_{\beta < \alpha} \om^{\beta}
			       & = \sum_{\beta < \gamma + 1} \om^{\beta} + \om^{\gamma+1} =
			      \begin{cases}
				      \om^{\gamma} \cdot 2 + \om^{\gamma + 1} & \text{ when $\gamma$ limit } \\
				      \om^{\gamma}  + \om^{\gamma + 1}        & \text{ otherwise }
			      \end{cases}                                    \\
			       & = \om^{\gamma + 1} = \om^{\alpha - 1} \, .
		      \end{align*}

		\item[For $\alpha$ a limit ordinal]
		      $\sum_{\beta < \alpha} \om^{\beta}
			      = \osup{\sum_{\beta < \gamma} \om^{\beta}}{\gamma < \alpha}$.
		      Let $\gamma < \alpha$, then $\gamma + 2 < \alpha$
		      and
		      $\sum_{\beta < \gamma} \om^{\beta} \leq
			      \sum_{\beta < \gamma + 2} \om^{\beta}$.
		      By induction hypothesis,
		      we conclude that
		      $\sum_{\beta < \gamma} \om^{\beta} \leq \om^{\gamma+1} <
			      \om^{\alpha - 1}$.
		      As a consequence,
		      $\sum_{\beta < \alpha} \om^{\beta}
			      \leq \om^{\alpha -
				      1}$.
		      Conversely, for every $\gamma < \alpha$,
		      $\om^\gamma \leq \sum_{\beta < \gamma+1} \om^{\beta}$,
		      and by definition of the ordinal exponentiation,
		      $\om^\alpha \leq \sum_{\beta < \alpha} \om^{\beta}$. \qedhere
	\end{itemize}
\end{proof}

\subsection{Proofs of \cref{sec-halpha}
	studiyng
	``The family $\FPhi{\alpha}$''
}
\begin{lemma}
	\label{hprod-product}
	Let $\alpha,\beta_1, \dots, \beta_n$ be ordinals,
	and $\beta = \om^{\beta_1} + \dots + \om^{\beta_n}$
	in Cantor Normal Form.
	Then,
	$\om^\alpha \hprod \beta = \om^{\alpha+\beta_1} + \cdots +
		\om^{\alpha+\beta_n}$.
\end{lemma}
\begin{proof}
	We proceed by induction on $\beta$:
	\begin{itemize}
		\item If $\beta = 0$ then $\om^\alpha \odot \beta = 0$.
		\item If $\beta = \gamma+1$ then
		      $\beta_n = 0$ and
		      $\gamma = \om^{\beta_1} + \dots + \om^{\beta_{n-1}}$.
		      Besides, by induction:
		      \[
			      \om^\alpha \odot (\gamma+1) = (\om^\alpha \odot \gamma) \oplus
			      \om^\alpha = \om^{\alpha+\beta_1} + \dots +
			      \om^{\alpha+\beta_{n-1}} + \om^{\alpha+0}
		      \]
		\item If $\beta$ is limit, then $\beta_n > 0$ and we proceed by
		      induction on $\beta_n$.

		      \begin{itemize}
			      \item If $\beta_n = \gamma+1$, then
			            $\beta = \sup_{n < \om} \om^{\beta_1} + \dots +
				            \om^{\beta_{n-1}} + \om^\gamma \cdot n$,
			            and thus by definition of $\odot$:
			            \begin{align*}
				            \om^\alpha \odot \beta & =
				            \sup_{n<\om} (\om^\alpha \odot (\om^{\beta_1} + \dots +
				            \om^{\beta_{n-1}} + \om^\gamma \cdot n))                                  \\
				                                   & = \sup_{n < \om} (\om^{\alpha+\beta_1} + \dots +
				            \om^{\alpha+\beta_{n-1}} + \om^{\alpha+\gamma} \cdot n)                   \\
				                                   & = (\om^{\alpha+\beta_1} + \dots +
				            \om^{\alpha+\beta_{n-1}} + \om^{\alpha+\gamma+1} )                        \\
				                                   & = (\om^{\alpha+\beta_1} + \dots +
				            \om^{\alpha+\beta_{n-1}} + \om^{\alpha+\beta_n} )
			            \end{align*}

			      \item If $\beta_n$ is limit then by definition of
			            $\om^{\beta_n}$,
			            $\beta = \sup_{\gamma < \beta_n} \om^{\beta_1} + \dots +
				            \om^{\beta_{n-1}} + \om^\gamma$,
			            and thus by definition of $\odot$:
			            \begin{align*}
				            \om^\alpha \odot \beta & =
				            \sup_{\gamma<\beta_n} (\om^\alpha \odot (\om^{\beta_1} + \dots +
				            \om^{\beta_{n-1}} + \om^\gamma ))                                                \\
				                                   & = \sup_{\gamma<\beta_n} (\om^{\alpha+\beta_1} + \dots +
				            \om^{\alpha+\beta_{n-1}} + \om^{\alpha+\gamma} )                                 \\
				                                   & = (\om^{\alpha+\beta_1} + \dots +
				            \om^{\alpha+\beta_{n-1}} + \om^{\alpha+\beta_n} )
				            \qedhere
				            \\
			            \end{align*}
		      \end{itemize}
	\end{itemize}
\end{proof}

We are now ready to prove the main lemma.
\canofam*
\begin{proof}[Proof of \cref{cano-fam}]
	We prove the result by induction on $\alpha$.

	\begin{itemize}
		\item It's immediate for $H_0$.
		\item Given $x \in H_1$, $H_1 \setminus \upc x$ is a finite set:
		      indeed, $x \in \Gamma_n$ for some $n < \om$ and thus
		      every $\Gamma_m$ for $m > n$ belong to $\upc x$.
		      It follows that $\h(H_1) \le \o(H_1) \le \om$ and since it is
		      infinite, $\om \le \h(H_1)$. Besides, $H_1$ contains arbitrary
		      large antichains and thus $\o(H_1) \ge \w(H_1) \ge \om$.
		      It follows that $\h(H_1) = \w(H_1) = \o(H_1) = \om^1$.

		\item If $\alpha >0$, \cite[Lemma 4.1]{dzamonja2020} and the induction hypothesis give:
		      \begin{align*}
			      \h(H_{\omega^\alpha}) = \o(H_{\omega^\alpha}) = \sum_{\beta <
				      \omega^\alpha} \omega^\beta \\
			      \w(H_{\omega^\alpha}) = \sup_{\beta < \omega^\alpha} \omega^\beta
		      \end{align*}

		      The second expression clearly evaluates to
		      $\omega^{\omega^\alpha}$ as desired.
		      Since $\om^\alpha$ is a limit ordinal,
		      \cref{sum-equals-sup-ordinals} immediatly gives
		      $\h(H_{\om^\alpha}) = \o(H_{\om^\alpha}) = \om^{\om^\alpha}$.

		\item For the last case: if
		      $\alpha = \om^{\alpha_1} + \cdots + \om^{\alpha_n}$ in CNF then
		      by  and the induction hypothesis:
		      \begin{equation*}
			      \h(H_{\alpha}) = \o(H_{\alpha}) =
			      \om^{\om^{\alpha_1}} \cdot \cdots \cdot \om^{\om^{\alpha_n}} =
			      \om^{\alpha}
		      \end{equation*}

		      For the width, {tab:fam:la-famille} gives
		      $\w(P \cdot Q) = \w(P) \odot \w(Q)$ (recall
		      that $\hprod$ is the Hessenberg product introduced
		      in Figure~\ref{fig:fam:ordinal-operations}).

		      It follows from \cref{hprod-product} that whenever $\alpha$ and $\beta$
		      are indecomposable, $\alpha \odot \beta = \alpha \cdot \beta$.
		      Now, by induction:
		      \[
			      \w(H_\alpha) = \om^{\om^{\alpha_1}} \odot \cdots \odot
			      \om^{\om^{\alpha_n}}
		      \]
		      Let's evaluate this expression from left to right:
		      $\om^{\om^{\alpha_1}}$ and $\om^{\om^{\alpha_2}}$ are both
		      indecomposable, therefore
		      \[
			      \om^{\om^{\alpha_1}} \odot \om^{\om^{\alpha_2}}
			      = \om^{\om^{\alpha_1}} \cdot \om^{\om^{\alpha_2}}
			      = \om^{\om^{\alpha_1} + \om^{\alpha_2}}
		      \]
		      The result is still indecomposable, so we can iterate with
		      $\om^{\om^{\alpha_3}}$, and so on.
		      In the end, these $\odot$'s are just usual ordinal product and we
		      get $\w(H_\alpha) = \om^{\om^\alpha}$. \qedhere
	\end{itemize}
\end{proof}

\section{Appendix to Section~\ref{sec:algebra-well-behaved} ``Elementary \wqos''}

\edgecasePfomk*
\begin{proof}
	\label{proof:prop-Pf-om-k}
	According to \cref{pf-mot}, $\o(\Pf(\om^{\times k+1}))\leq 2^{\om^{k+1}}=\om^{\om^k}$.

	We prove the lower bound by exhibiting a reflection.
	For any $\gamma\in \om^{\om^k}$, we can write $\gamma$ in CNF:
	$$\gamma = \om^{\alpha_1}\cdot a_1+\dots+ \om^{\alpha_n}\cdot a_n$$
	such that $0<a_1,\dots,a_n <\om$
	and $\om^k> \alpha_1>\dots >\alpha_n$.
	We note
	$c_i(\gamma)$ the first $i$ coefficients of the CNF of $\gamma$: $c_i(\gamma)\eqdef\sum_{j\in[1,i]}a_j$ for any $i\leq n$.
	Let $tip(\gamma)\eqdef \gamma - \om^{\alpha_1}\cdot a_1 = \om^{\alpha_2}\cdot a_2+\dots+ \om^{\alpha_n}\cdot a_n$.

	Since $\o(\om^{\times k})=\om^k$, there exists a reflection $g$ from
	$\om^k$ to $\om^{\times k}$.

	Then
	\begin{align*}
		f: \;\om^{\om^k} & \rightarrow \Pf(\om^{\times k+1})                                      \\
		\gamma           & \mapsto \setof{t_i\eqdef\left(c_i(\gamma),g(\alpha_i)\right)}{i\leq n}
	\end{align*}
	is a reflection.

	Consider $\gamma = \om^{\alpha_1}\cdot a_1+\dots+ \om^{\alpha_n}\cdot a_n$ and
	$\gamma' = \om^{\alpha'_1}\cdot a'_1+\dots+ \om^{\alpha'_m}\cdot a'_m$ in CNF, such that $f(\gamma)\hoareleq f(\gamma')$.
	By induction on $n$, let us show that $\gamma \leq \gamma'$:
	\begin{itemize}
		\item[Case $n=0$.] For $\gamma = 0$, $f(\gamma)=\emptyset \leq f(\gamma')$ for all $\gamma'<\om^{\om^k}$.
		\item[Case $n>0$.] There exists $j \in [1,m]$ such that $(c_1(\gamma),g(\alpha_1))\leq (c_j(\gamma'),g(\alpha'_j))$. Since $g$ is a reflection, then $\alpha_1 \leq \alpha'_j$. If $\alpha_1<\alpha'_j$ or $1<j$, then $\gamma <\gamma'$. Otherwise $j=1$ and $\alpha_1=\alpha'_1$, hence $c_1(\gamma)=a_1 \leq c_1(\gamma')=a'_1$. If $a_1<a'_1$ then $\gamma <\gamma'$.
		      Otherwise $a_1=a'_1$.
		      For all $i>1$, there exists $j\in[1,m]$ such that $(c_i(\gamma),g(\alpha_i))\leq (c_j(\gamma'),g(\alpha'_j))$, with $j\neq 1$ because $c_i(\gamma)>c_1(\gamma)=c_1(\gamma')$. Therefore $f(\gamma)\setminus \{(c_1(\gamma),g(\alpha_1))\} \hoareleq f(\gamma')\setminus(c_1(\gamma'),g(\alpha'_1))$, which means that $f(tip(\gamma))\hoareleq f(tip(\gamma))$ since $a_1=a'_1$. By induction hypothesis, $tip(\gamma)\leq tip(\gamma')$, therefore $\gamma \leq \gamma'$.
		      \qedhere
	\end{itemize}
\end{proof}

\edgecasePfomkalpha*
\begin{proof}
	\label{proof:pf-w-o-prod}
	Thanks to \cref{pf-width,om-k}
	we know that
	$
		\om^{\alpha\cdot\om^{k-1}}
		=
		2^{\w(X)}
		\leq \w(\Pf(X))
		\leq
		\o(\Pf(X))
	$.

	Therefore, to conclude, it suffices to bound
	$\o(\Pf(X))$ by $\om^{\om^{\alpha + (k-1)}}$.
	Let us prove this upper bound by induction over $k$. For simplicity's sake, we will initialize on $k=0$.

	\begin{itemize}
		\item [Induction property] For all $k\in\mathbb{N}$, $\o(Pf(X))<\om^{\om^{\alpha+k}}$. If $k>0$, $\o(Pf(X))=\om^{\om^{\alpha+(k-1)}}$.
		      The first half of the inductionproperty is what we need to call on as induction hypothesis in case $k>0$, the second half is the result we want to prove.
		\item[Case $k = 0$.]
		      If $X=\om^{\alpha}$ then $\Pf(X)\equiv\om^{\alpha}$, hence $\o(\Pf(X))<\om^{\om^{\alpha}}$.

		\item[Case $k > 0$.]
		      Observe that for all $Y\in\Pf(X)$, there exists $y\in X$ such that
		      $Y\hoareleq\{y\}$.
		      Let us use the
		      \kref{descent-equations}{descent equation} to conclude that
		      \begin{align*}
			      \o(\Pf(X))
			       & =
			      \osup{\o(\Pf(X)_{\not\hoaregeq Y}) + 1}{
				      Y \in \Pf(X)
			      }    \\
			       & =
			      \osup{\o(\Pf(X_{\not \geq y})) + 1}{
				      y\in X
			      }
		      \end{align*}

		      For all $\gamma<\alpha$, $x\in\om^{\times k}$,
		      \begin{align*}
			      X_{\not \geq (\gamma,x)} & \geqaug
			      \alpha_{\geq\gamma}\times \om^{\times k}_{\not \geq x} \;\sqcup\;
			      \alpha_{<\gamma}\times \om^{\times k} \\
			                               & \geqaug
			      \alpha\times \om^{\times k-1}\times \Gamma_l
			      \;\sqcup\;  \gamma \times \om^{\times k}
			      \text{ for some $ l\in \Nat $.}
		      \end{align*}
		      As a consequence,
		      \begin{equation*}
			      \Pf(X_{\not \geq (\gamma,x)}) \geqaug
			      (\Pf(\alpha\times \om^{\times k-1}))^{\times l}
			      \times \Pf(\gamma \times \om^{\times k})
		      \end{equation*}
		      Therefore,
		      $\o(\Pf(X_{\ngeq(\gamma,x)}))$
		      is bounded by the maximal order type of the right-hand side
		      of the inequality.

		      Remark that, on the one hand,
		      $\o(\Pf(\gamma \times \om^{\times k}))$
		      is at most
		      $2^{\o(\gamma \times \om^{\times k})}
			      =
			      2^{\gamma \otimes \om^k}$.
		      Now
		      $\gamma<\alpha$, and $\om^k<\alpha$, with $\alpha$ indecomposable, therefore
		      $\gamma \otimes \om^k<\alpha$ and $\o(\Pf(\gamma \times
				      \om^{\times
					      k}))<2^{\alpha}=\om^{\alpha}\leq\om^{\alpha\cdot\om^{k - 1}}$.
		      On the other hand, by induction hypothesis,
		      $\o(\Pf(\alpha\times \om^{\times k-1}))< \om^{\alpha\cdot\om^{k-1}}$.

		      Since
		      $\om^{\alpha\cdot\om^{k-1}}$ is
		      indecomposable,
		      we can conclude that
		      $\o(\Pf(X_{\nleq (x,\gamma)})) < \om^{\alpha\cdot\om^{k-1}}$.

		      Therefore
		      $\o(\Pf(X)) \leq \om^{\alpha\cdot\om^{k-1}}$. \qedhere
	\end{itemize}
\end{proof}

\edgecasePfomkepsilon*
\begin{proof}
	\label{proof:pf-o-epsilon}
	First let us prove that $\o(\Pf(X)) = \epsilon^{\om^k}$.
	We know $\o(X) = \epsilon \cdot \om^k$ hence $\o(\Pf(X))\leq 2^{\o(X)} = \epsilon^{\om^k}$.
	Therefore,  it suffices to prove
	by induction on $k \geq 0$
	that $\epsilon^{\om^k} \leq \o(\Pf(X))$.
	\begin{itemize}
		\item[Case $k=0$.]
		      We have $X = \epsilon$, hence $\Pf(X) \equiv \epsilon$
		      and $\o(\Pf(X)) = \epsilon = \epsilon^{\om^0}$ (we will deal with the width later).

		\item[Case $k>0$.]
		      For any $n<\om$ we define the following two sets
		      \begin{align*}
			      Y_n & \defined \setof{
				      (X_1,\dots,X_n)
				      \in
				      (\Pf(\epsilon \times \om^{\times k-1}))^{\times n}
			      }{
				      X_1 \hoareleq \dots \hoareleq X_n
			      }\;                                              \\
			      Z_n & \defined ((\Pf(\epsilon \times \om^{\times
				      k-1}))^{\times n}, \lexleq) \, .
		      \end{align*}

		      We will define two reflections $f$ and $g$ such that
		      $Z_n \ldefto{g} Y_n \ldefto{f} \Pf(X)$.
		      This immediately allows us to conclude that
		      $\o(\Pf(X))\geq \o(Y_n)\geq \o(Z_n)$.
		      Moreover, by induction hypothesis
		      $\o(Z_n) = \epsilon^{\om^{k-1}\cdot n}$,
		      hence $\o(\Pf(X))\geq \sup_n \epsilon^{\om^{k-1}\cdot n} = \epsilon^{\om^k}$.

		      \begin{enumerate}
			      \item
			            Let $f((X_1,\dots,X_n))\defined \bigcup_{i\leq n} \setof{(x,n-i)}{x\in X_i}$.
			            Let us prove that $f$ is a reflection.
			            Consider the following two elements of $Y_n$,
			            $y \defined (X_1, \dots, X_n)$ and $y' \defined (X_1', \dots, X_n')$.
			            Assume that $f(y) \leq f(y')$,
			            let us prove that $y \leq y'$.

			            Let $1 \leq i \leq n$,
			            and $x \in X_i$.
			            There exists $1 \leq j \leq n$ and $x' \in X_j'$
			            such that $(x,n-i) \leq (x', n-j)$.
			            Hence, $x \leq x'$ and $n-i \leq n-j$, therefore
			            $j \leq i$. As a consequence, and because
			            $X_1' \hoareleq \dots \hoareleq X_i'$, we have proven
			            that
			            $X_i \hoareleq \bigcup_{1 \leq j \leq i} X_j' \hoareleq
				            X_i'$.
			            Therefore $y \leq y'$ pointwise.

			      \item

			            To define $g$, let us first define $\pplus$ as the pointwise ordinal addition over elements of $\epsilon \times
				            \om^{\times k-1}$.
			            As usual, $\pplus$ lifts to $\Pf(\epsilon \times
				            \om^{\times k -1 })$
			            via $x \pplus Y \defined \setof{ x \pplus y}{y\in Y}$ for all $x\in \epsilon \times\om^{\times k-1}, Y \in \Pf(\epsilon \times \om^{\times k-1})$.

			            We also define $Y^{\top}$ for all $Y$ in $\Pf(\om^{\alpha}\times \om^{\times(k-1)})$ as the smallest element $x$ of $ \om^{\alpha}\times \om^{\times(k-1)}$ such that $y\leq x$ for all $y\in Y$. It can alternatively be defined and computed as the maximum component-wise of elements of $Y$. Observe that if $Y\equiv Y'$ then $Y^{\top}=Y'^{\top}$.

			            We are now ready to define $g$
			            through $g((X_1, \dots, X_n)) \defined
				            (X_1, X_1^{\top} + X_2, \dots, X_1^{\top} + \cdots +X_{n-1}^{\top} + X_n)$.

			            Let us prove that $g$ is a reflection.
			            Let $z = (X_1, \dots, X_n)$ and $z' = (X_1', \dots,
				            X_n')$
			            such that $g(z) \leq g(z')$.

			            Let us prove by induction on $1 \leq i \leq n$
			            that
			            $z \lexleq z'$.
			            Observe that $X_1 = g(z)_1 \hoareleq g(z')_1
				            = X_1'$.
			            Assume that
			            that $X_j \hoareeq X_j'$ for $1 \leq j < i$,
			            let us prove that $X_i \hoareleq X_i'$.
			            We know from $g(z) \leq g(z')$
			            that
			            $\sum_{1 \leq j < i} X_j^{\top} + X_i
				            \hoareleq
				            \sum_{1 \leq j < i} X_j'^{\top} + X_i'$.
			            However,
			            $\sum_{1 \leq j < i} X_j^{\top}
				            =
				            \sum_{1 \leq j < i} X_j'^{\top}$,
			            hence by component-wise left substraction
			            $X_i \hoareleq X_i'$.

			            We have proven that $g$ is a reflection.
		      \end{enumerate}
	\end{itemize}
	Therefore $\o(\Pf(X)) = \epsilon^{\om^k}$ is multiplicatively indecomposable.
	Since $\h(X)\leq 2^{\h(\epsilon \times \om^{\times k})} = \epsilon<\o(\Pf(X))$,
	according to \cref{kt}, $\w(\Pf(X))=\o(\Pf(X))$.
\end{proof}
